# Supplementary material for: Universal Scalings in 2D Anisotropic Dipolar Excitonic Systems
Source: arXiv:2106.04909 source file (2021-06-09)
Supplement: Supplementary file 1 [file paper2_Supp.pdf]

# Supplemental on-line material for
# Universal Scalings in 2D Anisotropic Excitonic Systems

Chern Chuang[1] and Jianshu Cao[1,*]

[1]*Department of Chemistry, Massachusetts Institute of Technology, MA 02139, USA*

[*] jianshu@mit.edu

## CONTENTS

S1. Derivation of Eq. (3) in the Main Text 3

A. Evaluation of $I_0(k)$ 3

B. Evaluation of $I_2(k)$ 4

C. Final Expression 4

D. Analysis of Higher Order Contributions 5

S2. Heuristic Derivation of Eq. (3) up to Linear Order 5

A. Interaction between 1D Chains in $k$ Space 7

B. From 1D to 2D 8

S3. Numerical convergence of dipole summation on a 2D lattice 8

S4. Approximate Derivation of $E^{0.5}$ Scaling of DOS 10

S5. Numerical Solution of the Coherent Potential Approximated Disorder-induced Absorption Linewidth 10

S6. Excitonic Couplings with Different Levels of Spatial Resolution in C8S3 Aggregates 12

S7. Construction of Helical-Rotationally Symmetric Tubular Aggregates of C8S3 12

S8. Derivation of Eq. (6) in the Main Text 16

S9. Finite Tube Extension of Eq. (6) in the Main Text 17

S10. Universality of Power-Law Exponents of DOS and $T$-Dependent Linewidth in Molecular Thin Films 18

S11. Radius Dependence of $T$-Dependent Linewidth of Tubular Dipolar Systems: 1D to 2D Transition 19

References 21

## S1. DERIVATION OF EQ. (3) IN THE MAIN TEXT

We first give the expressions of $I_0(k)$ and $I_2(k)$ in Eq. (2) in the main text, obtained by integrating over the $\phi$ coordinate:

$$I_0(k) = \int_{r_\mathrm{c}}^{\infty} dr \int_0^{2\pi} d\phi \cdot \frac{e^{ikr\cos\phi}}{r^2} = 2\pi \int_{r_\mathrm{c}}^{\infty} dr \frac{J_0(kr)}{r^2} \tag{S1}$$

$$I_2(k) = \int_{r_\mathrm{c}}^{\infty} dr \int_0^{2\pi} d\phi \cdot \frac{e^{ikr\cos\phi}\cos^2\phi}{r^2} = 2\pi \int_{r_\mathrm{c}}^{\infty} dr \frac{J_0(kr) - J_2(kr)}{2r^2} \tag{S2}$$

where $J_0(x)$ and $J_2(x)$ are the Bessel functions of the first kind.

We proceed to evaluate $I_0(k)$ and $I_2(k)$ in the small $k$ limit up to $k^2$.

### A. Evaluation of $I_0(k)$

$$\begin{aligned} I_0(k) &= 2\pi \int_{r_\mathrm{c}}^{\infty} dr \frac{J_0(kr)}{r^2} \\ &= \frac{2\pi}{r_\mathrm{c}} \left[ J_0(kr_\mathrm{c}) - kr_\mathrm{c} \int_{r_\mathrm{c}}^{\infty} dr \frac{J_1(kr)}{r} \right] \quad \text{(partial integration w.r.t. } r^{-2}\text{)} \\ &= \frac{2\pi J_0(kr_\mathrm{c})}{r_\mathrm{c}} + I_1(k) \end{aligned} \tag{S3}$$

The first term in Eq. (S3) follows

$$\frac{2\pi J_0(kr_\mathrm{c})}{r_\mathrm{c}} = \frac{2\pi}{r_\mathrm{c}} \left(1 - \frac{k^2 {r_\mathrm{c}}^2}{4}\right) + \mathcal{O}(k^4) \tag{S4}$$

The second term can be evaluated as

$$\begin{aligned} I_1(k) &= -2\pi k \left[ \int_0^{\infty} - \int_0^{r_\mathrm{c}} \right] dr \cdot \frac{J_1(kr)}{r} \\ &= -2\pi k \left(1 - \int_0^{r_\mathrm{c}} dr \frac{J_1(kr)}{r}\right) \\ &= -2\pi k \left(1 - \frac{kr_\mathrm{c}}{2}\right) + \mathcal{O}(k^3) \end{aligned} \tag{S5}$$

Combining the two terms we get

$$I_0(k) = \frac{2\pi}{r_\mathrm{c}} \left(1 - \alpha + \frac{\alpha^2}{4}\right) + \mathcal{O}(k^3) \tag{S6}$$

where we set $\alpha = k \cdot r_\mathrm{c}$.

### B. Evaluation of $I_2(k)$

$$I_2(k) = 2\pi \int_{r_c}^{\infty} dr \cdot \frac{J_0(kr) - J_2(kr)}{r^2} = \frac{I_0(k)}{2} - \pi \int_{r_c}^{\infty} dr \frac{J_2(kr)}{r^2} \tag{S7}$$

Similar to the treatment of $I_0(k)$, we integrate by part the second term and get

$$\begin{aligned} -\pi \int_a^{\infty} dr \frac{J_2(kr)}{r^2} &= -\frac{\pi}{r_c}\left[J_2(kr_c) + kr_c \int_{r_c}^{\infty} dr \frac{J_1(kr) - J_3(kr)}{r}\right] \\ &= -\frac{\pi J_2(kr_c)}{r_c} + I_3(k) \end{aligned} \tag{S8}$$

And

$$\begin{aligned} I_3(k) &= -\frac{\pi k}{2}\left[\int_0^{\infty} - \int_0^{r_c}\right] dr \cdot \frac{J_1(kr) - J_3(kr)}{r} \\ &= -\frac{\pi k}{2}\left[\left(1 - \frac{1}{3}\right) - \frac{kr_c}{2}\right] + \mathcal{O}(k^3) \end{aligned} \tag{S9}$$

Notice that the term proportional to $J_3(kr)$ scales at least as $k^3$.

Combining the two terms and evaluate to the order of $k^2$.

$$\begin{aligned} I_2(k) &= \frac{I_0}{2} - \frac{\pi J_2(kr_c)}{r_c} - \frac{\pi k}{2}\left(\frac{2}{3} - \frac{kr_c}{2}\right) + \mathcal{O}(k^3) \\ &= \frac{\pi}{r_c}\left[\left(1 - \alpha + \frac{\alpha^2}{4}\right) - \frac{\alpha^2}{8} - \left(\frac{\alpha}{3} - \frac{\alpha^2}{4}\right)\right] + \mathcal{O}(k^3) \\ &= \frac{\pi}{r_c}\left(1 - \frac{4\alpha}{3} + \frac{3\alpha^2}{8}\right) + \mathcal{O}(k^3) \end{aligned} \tag{S10}$$

### C. Final Expression

Substituting the expressions of $I_0(k)$ and $I_2(k)$ back into Eq. (2) in the main text, we have

$$\begin{aligned} E_c(\vec{k}) = \frac{\pi \mu_0^2}{A_0 r_c} \{ & \left(2 - 3\sin^2\theta_\mu\right) + \\ & \left[-2 + 2\sin^2\theta_\mu(2 - \sin^2\Delta)\right] \cdot (k \cdot r_c) + \\ & \left[\frac{1}{2} + \frac{3\sin^2\theta_\mu}{8}\left(-3 + 2\sin^2\Delta\right)\right] \cdot (k \cdot r_c)^2 \Big\} + \mathcal{O}(k^3) \end{aligned} \tag{S11}$$

which is Eq. (3) in the main text.

### D. Analysis of Higher Order Contributions

An estimate of the validity of Eq. (3), a second order Taylor expansion result, can be given by examining the next order contribution. In the case of expanding the continuum model, Eq. (1), one can show that the third order term vanishes, and the next order term is the fourth order:

$$\begin{aligned} E_{\rm c}(\vec{k}) = \bar{E}\,\{&(2-3\sin^2\theta_\mu) \\ &+[-2+2\sin^2\theta_\mu(2+\sin^2\Delta)]\cdot|k\cdot r_{\rm c}| \\ &+\left[\frac{1}{2}+\frac{3\sin^2\theta_\mu}{8}(-3+2\sin^2\Delta)\right]\cdot|k\cdot r_{\rm c}|^2 \\ &+\left[-\frac{1}{96}+\frac{\sin^2\theta_\mu}{192}(5-4\sin^2\Delta)\right]\cdot|k\cdot r_{\rm c}|^4\Big\} + \mathcal{O}(k^6) \end{aligned} \quad \text{(S12)}$$

In fact, all odd-power terms vanish, except for the linear one. Consequently, Eq. (3) describes the continuum model accurately up to the third order.

For the square lattices studied here, we find that $r_{\rm c} \approx a$ in general. Also, judging from Fig. 1(c), significant deviation between the exact lattice sum Eq. (1) and the second order expression Eq. (3) can be detected on the order of $|k \cdot a| \approx 0.5$. In contrast, Eq. (3) quantitatively agree (within 10%) with the exact continuum expression Eq. (2) up to $|k \cdot r_{\rm c}| \approx 1.5$, see a comparison between the two expressions shown in Fig.S1. We thus conclude that the range of validity of the second order expansion is larger than the range of validity of the continuum model itself. Consequently, the usefulness of the continuum model is mostly accounted for by Eq. (3).

## S2. HEURISTIC DERIVATION OF EQ. (3) UP TO LINEAR ORDER

We make use of our earlier result[1] on the dipolar coupling between homogeneous, parallel chains composed of equally spaced dipoles. We assume the chains lie within the $xy$-plane and are parallel to the $x$-axis with separation $D$ in the $y$-direction. The dipoles are given by $\vec{\mu} = \mu_0(\sin\theta\cos\phi, \sin\theta\sin\phi, \cos\theta)$. The interaction of between the $m$th site of the first chain $\vec{r}_m = (x_m, 0, 0)$ and the $n$th of the second $\vec{r}_n' = (x_n, D, 0)$ is given by

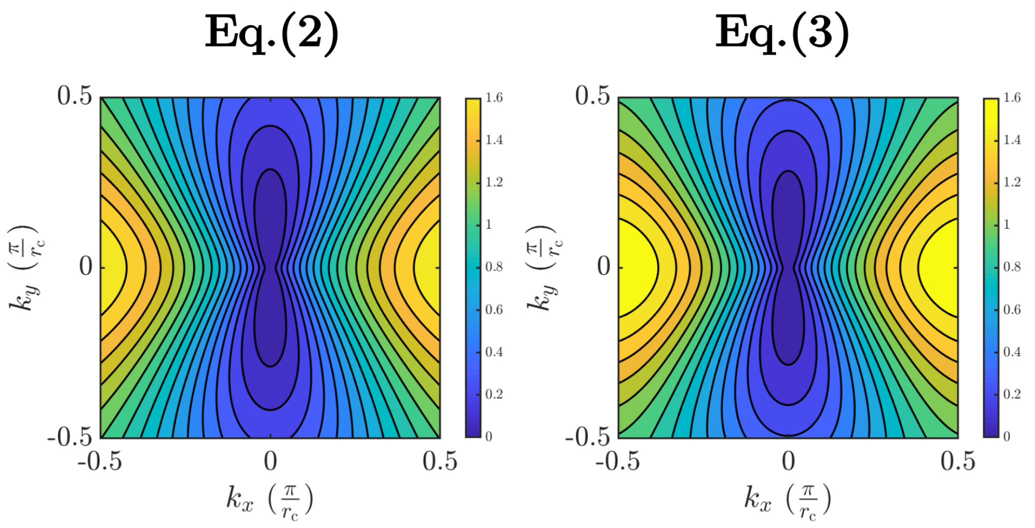


FIG. S1. Comparison between the continuum model, Eq. (2), (left) and its Taylor expansion up to second order, Eq. (3), (right). The energy scale is in $\bar{E} = \frac{2\pi\mu_0^2}{r_c A_0}$.

$$
\begin{aligned}
J_{mn} &= \frac{\mu_0^2}{r_{mn}^3} - \frac{3(\vec{r}_{mn}\cdot\vec{\mu}_m)^2}{r_{mn}^5} \\
&= \frac{\mu_0^2}{r_{mn}^3} - \frac{3\mu_0^2 \sin^2\theta[x_{mn}\cos\phi + D\sin\phi]^2}{r_{mn}^5} \\
&= \cos^2\theta \cdot J_{mn}^{(\mathrm{H,out})}(D) + \\
&\quad \sin^2\theta \cdot \left[\cos^2\phi J_{mn}^{(\mathrm{J})}(D) + \sin^2\phi\ J_{mn}^{(\mathrm{H,in})}(D) + \sin 2\phi\ J_{mn}^{(\mathrm{M})}(D)\right]
\end{aligned} \tag{S13}
$$

where $x_{mn} = x_m - x_n$ and the individual $J^{(\mathrm{x})}$ terms are defined as

$$
\begin{aligned}
J_{mn}^{(\mathrm{H,out})}(D) &= \frac{\mu_0^2}{(x_{mn}^2 + D^2)^{3/2}} \\
J_{mn}^{(\mathrm{J})}(D) &= \frac{\mu_0^2(-2x_{mn}^2 + D^2)}{(x_{mn}^2 + D^2)^{5/2}} \\
J_{mn}^{(\mathrm{H,in})}(D) &= \frac{\mu_0^2(x_{mn}^2 - 2D^2)}{(x_{mn}^2 + D^2)^{5/2}} \\
J_{mn}^{(\mathrm{M})}(D) &= -\frac{3\mu_0^2 D x_{mn}}{(x_{mn}^2 + D^2)^{5/2}}
\end{aligned}
$$

For a schematic drawing of the system geometry and relevant variables please see Figs. 1(b) or S2.

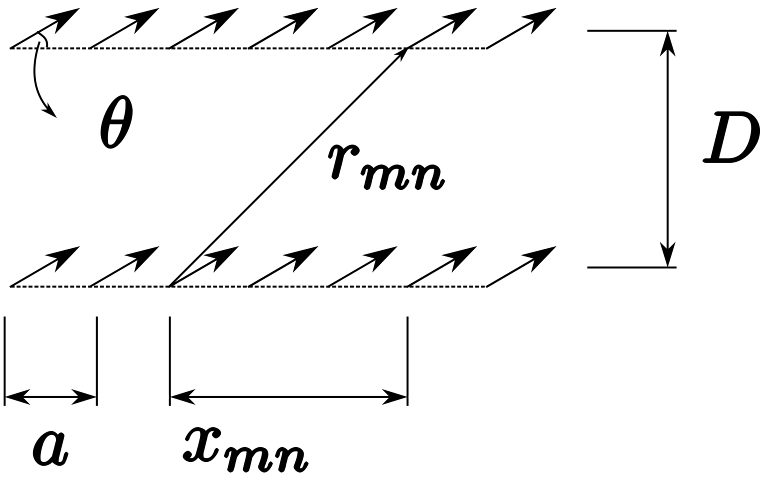


FIG. S2. Schematic representation of two interacting dipole chains.

### A. Interaction between 1D Chains in $k$ Space

We are interested in the coupling matrix element in the momentum space. This amounts to calculating the following quantity:

$$
\begin{aligned}
J_{kl} = \delta_{kl} J_{kk} &= \sum_{n=1}^{N} \sum_{m=1}^{N} J_{mn} e^{2\pi i k x_{mn}} \\
&\approx \frac{2}{Na^2} \int_0^{Na} dx \; (Na - x) \cos(2\pi k x) J(x)
\end{aligned} \tag{S14}
$$

where in the first line we take advantage of the translational symmetry, and the continuum approximation is invoked in the second line. $a > 0$ is the lattice spacing. In particular, we focus on the case where $k = 0$.

$$
\begin{aligned}
J_{k=0}^{(\mathrm{H,out})}(D) &= \frac{2\mu_0^2}{Na^2} \frac{-D + \sqrt{D^2 + N^2 a^2}}{D^2} \\
J_{k=0}^{(\mathrm{J})}(D) &= \frac{2\mu_0^2}{Na^2} \left( \frac{1}{D} - \frac{1}{\sqrt{D^2 + N^2 a^2}} \right) \\
J_{k=0}^{(\mathrm{H,in})}(D) &= -\frac{2\mu_0^2 N}{D^2 \sqrt{D^2 + N^2 a^2}} \\
J_{k=0}^{(\mathrm{M})}(D) &= 0
\end{aligned}
$$

Furthermore, we are interested in the infinite chain limit ($N \to \infty$), which leads to the following.

$$
J_{k=0}^{(\mathrm{H,out})}(D) = -J_{k=0}^{(\mathrm{H,in})} = \frac{2\mu_0^2}{aD^2} \tag{S15}
$$

$$
J_{k=0}^{(\mathrm{J})}(D) = J_{k=0}^{(\mathrm{M})}(D) = 0 \tag{S16}
$$

### B. From 1D to 2D

With the above expressions, we need to further Fourier transform the other dimension ($D$, along the $y$-axis) to obtain the 2D dispersion. Notice that the only nontrivial $D$ dependence is inverse square, one has

$$\begin{aligned}E_{k_x=0}(k_y) &= \frac{1}{a'}\left(\int_{-\infty}^{-a'} + \int_{a'}^{\infty}\right) dy\ e^{2\pi i k_y y}\ J_{k=0}(y) \\ &\propto 2\int_{a'}^{\infty} dy\ \frac{\cos(2\pi k_y y)}{y^2} \\ &= -\frac{\pi k_y}{2} + \frac{\cos(k_y a')}{a'} + k_y \mathrm{Si}(k_y a') \\ &= \frac{1}{a'} - \frac{\pi k_y}{2} + \mathcal{O}(k_y^2) \end{aligned} \tag{S17}$$

where $\mathrm{Si}(x) = \int_0^x dt \sin(t)/t$ is the sine integral function.

Combining Eqs. (S13) and (S17), the scaling of the full 2D dispersion as a function of the azimuth angle in the $k$-space ($\phi_k = \arctan\frac{k_y}{k_x}$) in the small $k = \sqrt{k_x^2 + k_y^2}$ regime is given by

$$E(k, \phi_k) - E(0) = \frac{\pi\mu_0^2}{2A_0}\left[-\cos^2\theta + \sin^2\theta\cos^2(\phi - \phi_k)\right]\cdot k + \mathcal{O}(k^2) \tag{S18}$$

where $A_0 = aa'$ is the share of area occupied by a dipole. This agrees with Eq. (3) in the main text up to linear order.

## S3. NUMERICAL CONVERGENCE OF DIPOLE SUMMATION ON A 2D LATTICE

In the main text we compare the continuum model with the results of exact numerical Fourier summation, Eq. (1). In practice the summation is truncated at a certain cutoff radius $R$:

$$E(\vec{k}; R) = {\sum_{|\vec{r}_n|<R}}' J(\vec{r}_n) e^{i\vec{k}\cdot\vec{r}_n} \tag{S19}$$

where we set the site energy $E_0$ to zero and $\mu_0 = a = 1$ for convenience.

The convergence of this expression is expected to be worst for $\vec{k} = 0$, where we have the square lattice dipole summation $E(0; R) = {\sum_{|\vec{r}_n|<R}}' J(\vec{r}_n)$. It has been shown that the value of $E(0; R \to \infty) = E(0) = 4\zeta(3/2)\beta(3/2)(1 - 3\sin^2\theta_\mu/2) \approx 9.0336 \cdot (1 - 3\sin^2\theta_\mu/2)$,[2]

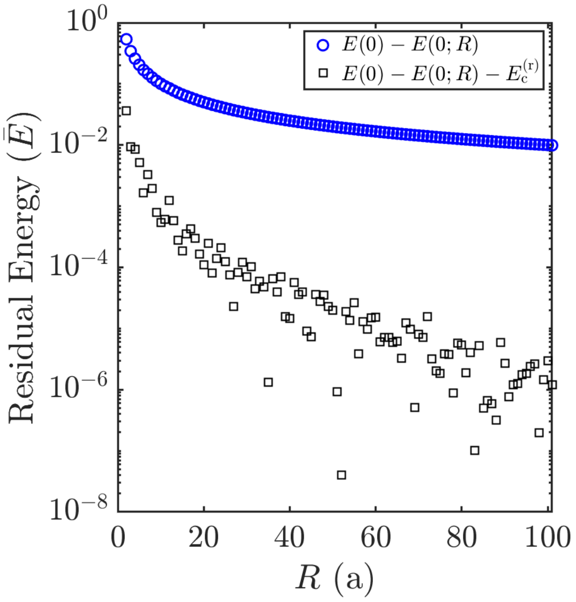


FIG. S3. The convergence of $E(0;R)$ and $E(0;R) + E_c^{(r)}(0;R)$ to their asymptotic value $E(0) \approx 4.568$.

where $\zeta(x)$ is the Riemann zeta function and $\beta(x)$ is the Dirichlet series[3]

$$\beta(x) = \sum_{n=0}^{\infty} \frac{(-1)^n}{(2n+1)^x} \tag{S20}$$

In Fig. S3 we show the convergence of $E(0;R)$ of the in-plane configuration $\theta_\mu = \pi/2$ towards $E(0) \approx 4.568$ as a function of $R$, which can be shown to be proportional to $R^{-1}$. In practice, the exact result is replaced by a lattice sum with a finite $R$ in addition to a continuum approximated residual energy given by Eq. (3), similar to the Ewald sum with a step-function cut-off and applied to all values of $\vec{k}$. For $k = 0$ the residual energy is

$$E_c^{(r)}(0;R) = -\frac{1 + 3\cos 2\theta_\mu}{2R}\bar{E} \tag{S21}$$

where $\bar{E} = \pi\mu^2/A_0 = \pi$ as in the main text. In Fig. S3 we also show the convergence of $E(0;R) + E_c^{(r)}(0;R)$, which is at least two orders of magnitude smaller than the truncated dipole sum alone. In the main text all calculations were carried out with $R = 50a$ and exact numerical evaluation of Eq.(2) by setting $r_c = R$.

## S4. APPROXIMATE DERIVATION OF $E^{0.5}$ SCALING OF DOS

Here we provide an approximate derivation of the $E^{0.5}$ scaling of DOS for the in-plane $\theta_\mu = \pi/2$ configuration. Rewriting Eq. (3) of the main text as

$$\frac{E(\vec{k}) - E(0)}{\bar{E}} = 2\cos^2\phi_k \cdot \bar{k} + \frac{1 - 6\cos^2\phi_k}{8} \cdot \bar{k}^2 \tag{S22}$$

$$= 2\frac{k_x^2}{\sqrt{k_x^2 + k_y^2}} + \frac{-5k_x^2 + k_y^2}{8} \tag{S23}$$

where in the first line we assume $\phi_\mu = 0$ without loss of generality ($\Delta = \phi_k$) and write $\bar{k} = k \cdot r_c$. In the second line we write $k_x = \bar{k}\cos\phi_k$ and $k_y = \bar{k}\sin\phi_k$.

We next approximate Eq. (S23) to make the calculation of DOS more tractable while still maintaining the qualitative features of the anisotropic dispersion: (1) We replace the linear term with $k_x$ and (2) the quadratic term with $k_y^2$.

$$\frac{E(\vec{k}) - E(0)}{\bar{E}} \approx 2k_x + \frac{k_y^2}{8} \tag{S24}$$

This is essentially linearizing the angular dependence $\phi_k$ in scaling between the dominantly linearly dispersed $k_x$ direction and the purely quadratically dispersed $k_y$ direction. From here, it is straightforward to calculate the $k$ space area covered within the isoenergetic contour $E(\vec{k}) - E(0) = E'$ in the first quadrant:

$$A(E') = \int_0^{k_{y,\max}} k_x \, dk_y = \frac{E' \cdot k_{y,\max}}{2} - \frac{k_{y,\max}^3}{48} = \frac{(8E')^{3/2}}{24} \tag{S25}$$

where $k_{y,\max} = \sqrt{8E'}$ is the maximal $k_y$ given $E'$. It follows that

$$\mathrm{DOS}(E) = \frac{dA}{dE} \propto E^{1/2} \tag{S26}$$

## S5. NUMERICAL SOLUTION OF THE COHERENT POTENTIAL APPROXIMATED DISORDER-INDUCED ABSORPTION LINEWIDTH

Here we present the result of disorder-induced absorption linewidth by numerically solving the self-consistent equation for the self-energy under the coherent potential approximation[4]:

$$\Sigma(\omega) = \left[\int dx \frac{P(x)x}{1 - (x - \Sigma(\omega))g_0(\omega)}\right] \cdot \left[\int dx \frac{P(x)}{1 - (x - \Sigma(\omega))g_0(\omega)}\right]^{-1} \tag{S27}$$

where $P(x) = \exp\left(-x^2/2\sigma^2\right)/\sqrt{2\pi\sigma^2}$ is the distribution function of the on-site disorder, taken to be a Gaussian in our case and

$$g_0(\omega) = \frac{1}{N}\sum_k \frac{1}{\omega - E_k - \Sigma(\omega) + i\eta}$$

is the averaged Green's function, where $\eta$ is a small positive constant. Iteratively solving Eq. (S27) using the dispersion Eq. (3) for $E_k$ and different values of $\sigma$ leads to the results shown in Fig. S4, where the power-law fitting of $\sigma^{2.74}$ agrees well with the result of direct diagonalization shown discussed in the main text, Fig. 3(a).

## S6. EXCITONIC COUPLINGS WITH DIFFERENT LEVELS OF SPATIAL RESOLUTION IN C8S3 AGGREGATES

In the main text we adopt realistic models of excitonic coupling between representative dye molecule C8S3: Simple dipole, extended dipole, and atomic transition charges. The former two have been documented in the literature[5] and reiterate as follows.

$$J_{\text{sd}}(\vec{n}-\vec{m}) = \frac{\mu_0^2}{r_{nm}^3}\left[1 - 3(\hat{\mu}_n \cdot \hat{r}_{nm})(\hat{\mu}_m \cdot \hat{r}_{nm})\right] \tag{S28}$$

$$J_{\text{ed}}(\vec{n}-\vec{m}) = q^2\left(\frac{1}{r_{nm}^{++}} + \frac{1}{r_{nm}^{--}} - \frac{1}{r_{nm}^{+-}} - \frac{1}{r_{nm}^{-+}}\right) \tag{S29}$$

where $\mu_0 = 11.4$ Debye, $q = 0.34e$ ($e$ is the electron charge), and

$$r_{nm}^{\pm\pm} = |\vec{r}_{nm} \pm l(\hat{\mu}_n - \hat{\mu}_m)|$$

$$r_{nm}^{-+} = |\vec{r}_{nm} - l(\hat{\mu}_n + \hat{\mu}_m)|$$

$$r_{nm}^{+-} = |\vec{r}_{nm} + l(\hat{\mu}_n + \hat{\mu}_m)|$$

where $l = 7\mathring{A}$.

The method atomic transition charges assume that the transition density between, in our case, the ground and the first excited state of a molecule to be condensed onto the positions of its constituent atoms.[6] Thus, it is in a sense similar to the extended dipole method but now the summation between interacting charges runs through, in this case, all 108-by-108 atom pairs between two C8S3 molecules. We first optimize the ground state geometry of a C8S3 molecule with the semi-empirical PM7 force field and perform ZINDO calculation to obtain its first excited state transition density atomic transition charges.[7] The parameters are given in Tables I and II. The molecule is aligned such that the transition moment is along the $y$-axis and the $x$-axis is normal to the aromatic group.

| # | Atom | x | y | z | c | # | Atom | x | y | z | c |
|---|---|---|---|---|---|---|---|---|---|---|---|
| 1 | C | -0.0062 | -6.0436 | 0.7011 | -0.0121 | 28 | H | 6.0475 | -3.3460 | -3.9571 | -0.0003 |
| 2 | C | 0.0319 | -4.6716 | 0.4270 | 0.0101 | 29 | H | 5.4180 | -2.8106 | -5.5175 | -0.0010 |
| 3 | C | -0.2671 | -4.1652 | -0.8791 | -0.0018 | 30 | C | 6.0025 | -4.9058 | -5.4716 | -0.0002 |
| 4 | C | -0.5974 | -5.0199 | -1.9359 | -0.0097 | 31 | H | 5.9968 | -5.7516 | -4.7554 | 0.0008 |
| 5 | C | -0.6194 | -6.3806 | -1.6477 | -0.0294 | 32 | H | 5.3629 | -5.2233 | -6.3179 | 0.0001 |
| 6 | C | -0.3314 | -6.8838 | -0.3582 | -0.0145 | 33 | C | 7.4267 | -4.6588 | -5.9644 | -0.0008 |
| 7 | H | 0.1951 | -6.4613 | 1.7431 | -0.0037 | 34 | H | 8.0948 | -4.3821 | -5.1405 | -0.0000 |
| 8 | H | -0.8277 | -4.6447 | -2.9288 | -0.0050 | 35 | H | 7.8429 | -5.5562 | -6.4353 | -0.0001 |
| 9 | C | 0.2033 | -2.3733 | 0.4971 | -0.0337 | 36 | H | 7.4646 | -3.8507 | -6.7031 | -0.0003 |
| 10 | N | -0.1988 | -2.7432 | -0.8131 | -0.0576 | 37 | C | 0.7357 | -3.6343 | 2.6707 | 0.0008 |
| 11 | N | 0.3300 | -3.5480 | 1.2477 | -0.0776 | 38 | H | 1.6037 | -4.3787 | 2.7465 | -0.0040 |
| 12 | C | -0.0920 | -1.8947 | -2.0176 | 0.0008 | 39 | H | 1.1500 | -2.6569 | 3.0001 | -0.0047 |
| 13 | H | -0.7025 | -2.3566 | -2.8279 | -0.0019 | 40 | C | -0.4384 | -4.0647 | 3.5658 | -0.0014 |
| 14 | H | -0.5654 | -0.9040 | -1.7880 | -0.0073 | 41 | H | -1.0877 | -4.7961 | 3.0292 | 0.0012 |
| 15 | C | 1.3600 | -1.6894 | -2.4740 | -0.0000 | 42 | H | -1.0843 | -3.1934 | 3.7870 | -0.0029 |
| 16 | H | 1.3875 | -0.8208 | -3.1770 | -0.0065 | 43 | C | 0.0520 | -4.6990 | 4.8577 | -0.0007 |
| 17 | H | 1.9928 | -1.4001 | -1.6093 | -0.0005 | 44 | H | -0.7950 | -4.9153 | 5.5295 | -0.0023 |
| 18 | C | 1.9504 | -2.9265 | -3.1577 | 0.0002 | 45 | H | 0.7047 | -4.0187 | 5.4266 | -0.0019 |
| 19 | H | 1.9446 | -3.7850 | -2.4537 | 0.0041 | 46 | S | 0.9429 | -6.2343 | 4.4884 | -0.0010 |
| 20 | H | 1.3141 | -3.2343 | -4.0095 | -0.0003 | 47 | O | 1.0638 | -6.9491 | 5.7617 | -0.0030 |
| 21 | C | 3.3832 | -2.6672 | -3.6420 | -0.0006 | 48 | O | 0.1022 | -6.9103 | 3.4508 | -0.0002 |
| 22 | H | 4.0205 | -2.3659 | -2.7871 | -0.0004 | 49 | O | 2.2196 | -5.7505 | 3.8861 | -0.0016 |
| 23 | H | 3.3992 | -1.8158 | -4.3482 | -0.0024 | 50 | C | 0.4002 | -1.0887 | 1.0279 | -0.0274 |
| 24 | C | 3.9767 | -3.9134 | -4.3130 | 0.0001 | 51 | H | 0.7627 | -1.0698 | 2.0651 | -0.0053 |
| 25 | H | 3.9716 | -4.7617 | -3.5995 | 0.0014 | 52 | C | 0.1468 | 0.1395 | 0.4263 | -0.0109 |
| 26 | H | 3.3370 | -4.2299 | -5.1589 | 0.0001 | 53 | H | -0.2382 | 0.1462 | -0.6067 | -0.0002 |
| 27 | C | 5.4072 | -3.6573 | -4.8054 | -0.0004 | 54 | C | 0.3221 | 1.3478 | 1.0728 | 0.0436 |

TABLE I. Transition density condensed to each of the 108 atoms in a C8S3 molecule.

| # | Atom | x | y | z | c | # | Atom | x | y | z | c |
|---|---|---|---|---|---|---|---|---|---|---|---|
| 55 | H | 0.6057 | 1.3297 | 2.1311 | 0.0070 | 82 | C | -1.7297 | -0.5290 | -7.0668 | 0.0002 |
| 56 | C | 0.1132 | 2.6390 | 0.5358 | 0.0233 | 83 | H | -2.3793 | 0.3157 | -7.3677 | -0.0011 |
| 57 | C | 0.0573 | 4.4675 | -0.8641 | 0.0022 | 84 | H | -2.3701 | -1.1952 | -6.4572 | 0.0012 |
| 58 | C | -0.3574 | 4.8872 | 0.4396 | -0.0054 | 85 | C | -1.2413 | -1.2784 | -8.3146 | 0.0000 |
| 59 | N | -0.2981 | 3.7436 | 1.2822 | 0.0740 | 86 | H | -0.5906 | -2.1237 | -8.0162 | 0.0011 |
| 60 | N | 0.3635 | 3.0826 | -0.7792 | 0.0620 | 87 | H | -0.6070 | -0.6112 | -8.9305 | -0.0007 |
| 61 | C | 0.1224 | 5.3686 | -1.9359 | 0.0088 | 88 | C | -2.4074 | -1.7980 | -9.1523 | 0.0001 |
| 62 | C | -0.2336 | 6.6821 | -1.6587 | 0.0296 | 89 | H | -3.0536 | -0.9822 | -9.4959 | -0.0005 |
| 63 | C | -0.6507 | 7.0998 | -0.3699 | 0.0160 | 90 | H | -2.0505 | -2.3308 | -10.0407 | 0.0001 |
| 64 | H | 0.4333 | 5.0577 | -2.9290 | 0.0049 | 91 | H | -3.0348 | -2.4940 | -8.5834 | 0.0005 |
| 65 | C | -0.7275 | 6.2155 | 0.6964 | 0.0109 | 92 | C | -0.7011 | 3.7353 | 2.7082 | -0.0007 |
| 66 | H | -1.0997 | 6.5310 | 1.7252 | 0.0040 | 93 | H | -0.0158 | 3.0807 | 3.2836 | 0.0049 |
| 67 | C | 0.8164 | 2.2784 | -1.9306 | -0.0010 | 94 | H | -0.5658 | 4.7996 | 3.1092 | 0.0024 |
| 68 | H | 1.5817 | 2.8698 | -2.4891 | 0.0019 | 95 | C | -2.1681 | 3.3001 | 2.8765 | 0.0013 |
| 69 | H | 1.3367 | 1.3645 | -1.5591 | 0.0063 | 96 | H | -2.7459 | 3.5041 | 1.9435 | -0.0006 |
| 70 | C | -0.3624 | 1.9194 | -2.8489 | 0.0012 | 97 | H | -2.2205 | 2.2046 | 3.0274 | 0.0041 |
| 71 | H | -0.9388 | 2.8340 | -3.1053 | -0.0026 | 98 | C | -2.8333 | 4.0268 | 4.0342 | 0.0008 |
| 72 | H | -1.0853 | 1.2744 | -2.3108 | 0.0030 | 99 | H | -3.8049 | 3.5632 | 4.2749 | 0.0030 |
| 73 | C | 0.1278 | 1.2367 | -4.1292 | 0.0003 | 100 | H | -2.2467 | 3.9534 | 4.9629 | 0.0014 |
| 74 | H | 0.7417 | 1.9405 | -4.7246 | -0.0013 | 101 | S | -3.0942 | 5.7667 | 3.5985 | 0.0007 |
| 75 | H | 0.8049 | 0.3853 | -3.8775 | 0.0038 | 102 | O | -3.8263 | 5.7426 | 2.3176 | -0.0005 |
| 76 | C | -1.0462 | 0.7282 | -4.9752 | 0.0005 | 103 | O | -3.7916 | 6.3596 | 4.7429 | 0.0028 |
| 77 | H | -1.6932 | 1.5779 | -5.2712 | -0.0016 | 104 | O | -1.6852 | 6.2840 | 3.3937 | -0.0000 |
| 78 | H | -1.6912 | 0.0606 | -4.3716 | 0.0021 | 105 | Cl | -1.0694 | 8.7420 | -0.1408 | 0.0050 |
| 79 | C | -0.5547 | -0.0135 | -6.2255 | 0.0006 | 106 | Cl | -0.1663 | 7.8418 | -2.9254 | 0.0064 |
| 80 | H | 0.0788 | 0.6575 | -6.8375 | -0.0011 | 107 | Cl | -0.3918 | -8.5747 | -0.1097 | -0.0046 |
| 81 | H | 0.0974 | -0.8592 | -5.9329 | 0.0019 | 108 | Cl | -1.0107 | -7.4845 | -2.9066 | -0.0063 |

TABLE II. Transition density condensed to each of the 108 atoms in a C8S3 molecule (continued).

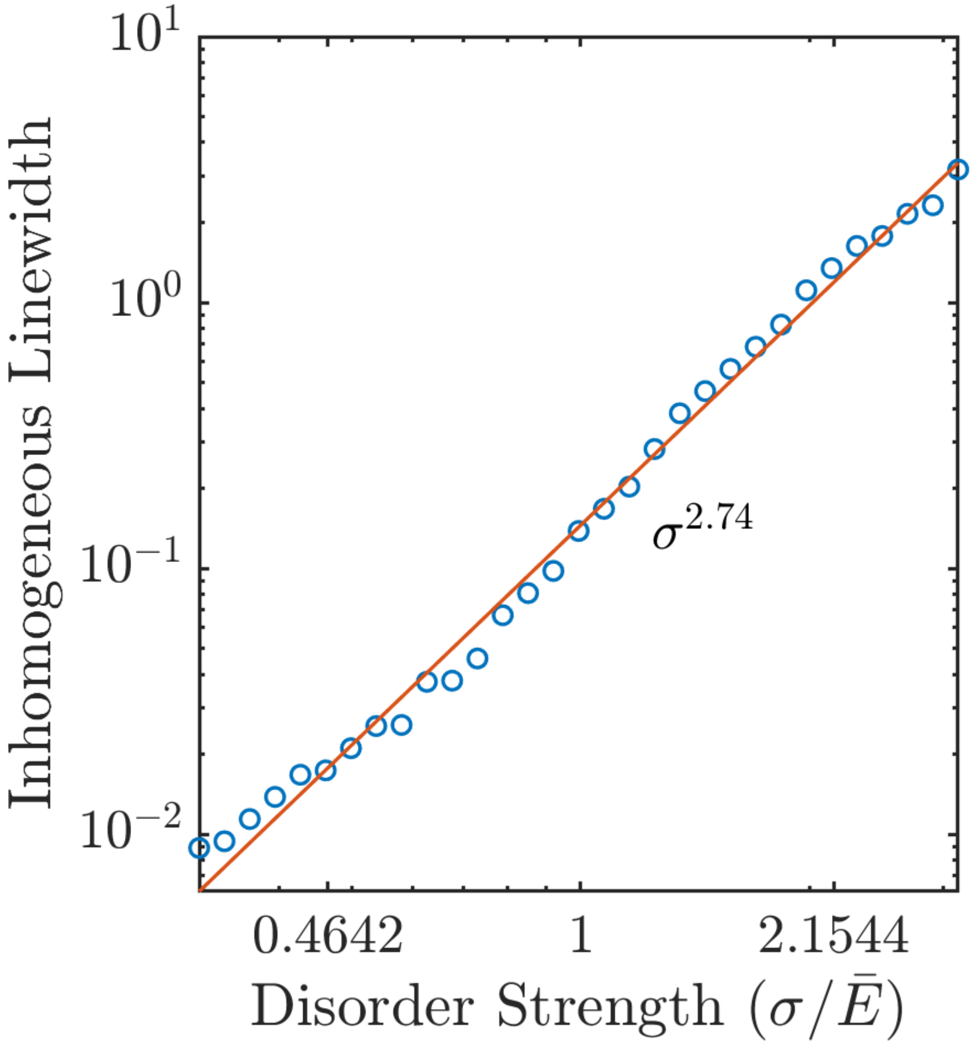


FIG. S4. Numerical solution to the self-consistent Eq. (S27). The line is the power-law fit to the data with exponent 2.74. The range of disorder strength is chosen to match the range in Fig. 3(a) that shows the $\sigma^{2.8}$ scaling.

## S7. CONSTRUCTION OF HELICAL-ROTATIONALLY SYMMETRIC TUBULAR AGGREGATES OF C8S3

In the main text we analyze the energy gap between the perpendicular- and the parallel-polarized peaks of helical-rotationally symmetric tubular aggregates. We follow the recipe provided by Knoester et al.[8], where the locations and the direction of the transition dipole

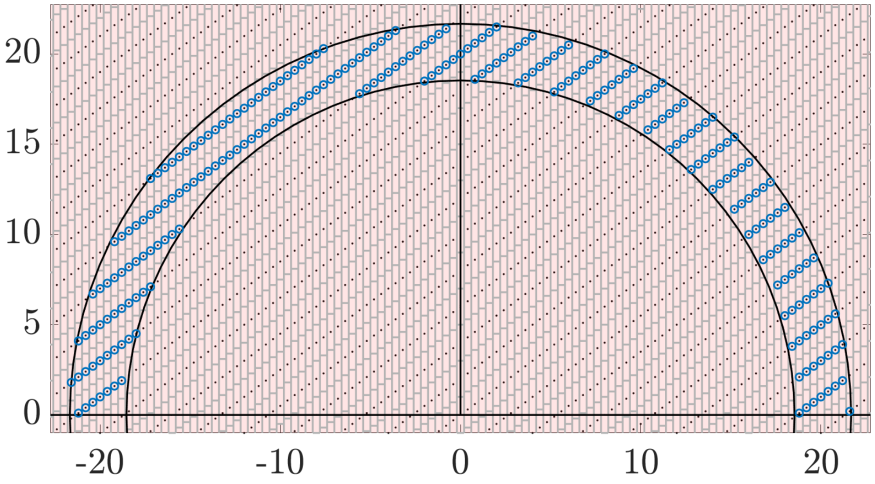


FIG. S5. All possible unique chiral vectors (black dots in the upper two quadrants) for a 20-by-4 Å brick tiling with a slip of 3 Å between neighboring bricks. Further specifying a constraint on the radii of the resulting tubes to be $29.5 \leq r \leq 34.5$ Å leads to those marked with blue circles. The tick labels are measured in nm.

moment of a stacked ring tubular aggregate are given by

$$\vec{r}(n_1, n_2) = [r\cos(n_1\gamma, n_2\phi_2), r\sin(n_1\gamma, n_2\phi_2), n_1 h]$$
$$\vec{\mu}(n_1, n_2) = [-\sin\theta' \sin(n_1\gamma + n_2\phi_2), \sin\theta' \cos(n_1\gamma + n_2\phi_2), \cos\theta'] \tag{S30}$$

where $(n_1, n_2)$ are integers with $n_1 \in (-\infty, \infty)$ labelling the ring number and $n_2 \in [1, N_2]$ labelling the unit cell within a ring, where $N_2$ is the rotational symmetry number. ($\theta'$ refers to $\theta$ in Ref.[8].) $\phi_2 = 2\pi/N_2$, $\gamma$ is the offset of the first unit cell in a ring compared to its correspondence in the preceding ring, $r$ is the radius of the tube, and $h$ is the separation between adjacent rings.

To properly enumerate over possible tubular aggregate configurations, we start from tiling the 2D plane with rectangular bricks. A unique 2D plane can be specified by a slip parameter given the dimensions of the brick (the length and width of the monomer projected to the plane of aggregation). One exemplar 2D configuration is shown in Fig. S5 with a rectangular brick dimension 20-by-4 Å and slip parameter 0.3 Å.

Once a 2D planar configuration is specified, one can then designate a chiral vector that specifies the way a 2D sheet is folded into an infinitely long cylinder, a concept first conceived in the study of carbon nanotubes.[9] In Fig. S5, we mark all unique chiral vectors with lengths

(diameters of the corresponding cylinder) falling within the range $2\pi(32 \pm 2.5)$ $\mathring{A}$, in accordance with the dimension of the inner tube of the C8S3 double-wall tubular aggregate.[10] Given the 2D plane and the chiral vector, one can retrieve the corresponding parameters needed in Eq. (S30).

The above information suffices for one to calculate the exciton dispersion for point dipole interactions among the monomers, as presented as the red dots in Fig. 3 in the main text. To calculate the dispersions for the extended dipole and transition charges interactions, similar procedures with additional details about the internal structure within a unit cell can be employed. The computer routines responsible for generating Fig. 3 in the main text are available upon request.

## S8. DERIVATION OF EQ. (6) IN THE MAIN TEXT

Here we provide the derivation of Eq. (6) in the main text. We again make use of our previous results on the interaction matrix element between parallel dipole chains in the Bloch basis.[1] As we are interested in the dispersion along the circumferential direction of tubular excitonic aggregates, it suffices to consider only the $k = 0$ Bloch states of the parallel stripes, see Fig. S6. We also limit ourselves to the case where all dipoles lie within the plane of aggregation (tangent to the cylindrical surface). Now, the energy gap under consideration can be expressed as

$$E(0, \pm 1) - E(0, 0) = \frac{2\mu_0^2}{A_0} \int_0^\pi r \; d\phi \; (\cos\phi - 1) \left[ J_\parallel(d, \phi) - J_\perp(d, \phi) \right] \tag{S31}$$

where $d$ is the separation between the two stripes in the integrand, see Fig. S6 for a schematic drawing. $J_\parallel(x)$ $[J_\perp(x)]$ is the said $k = 0$ matrix element between chains with dipoles parallel (perpendicular) to the vector $\vec{x}$ that separates the two chains.

$$d(\phi) = r\sqrt{2 - 2\cos\phi} \tag{S32}$$

$$J_\parallel(x, \phi) = -\frac{2}{x^2} \sin^2\beta \cos^2\frac{\phi}{2} \tag{S33}$$

$$J_\perp(x, \phi) = \frac{2}{x^2} \sin^2\beta \sin^2\frac{\phi}{2} \tag{S34}$$

Note that in particular $J_\perp(x)$ is the same as $J_{k=0}^{(\mathrm{H,out})}(D)$ in Eq. (S15), where we have taken the limit of infinite chain.

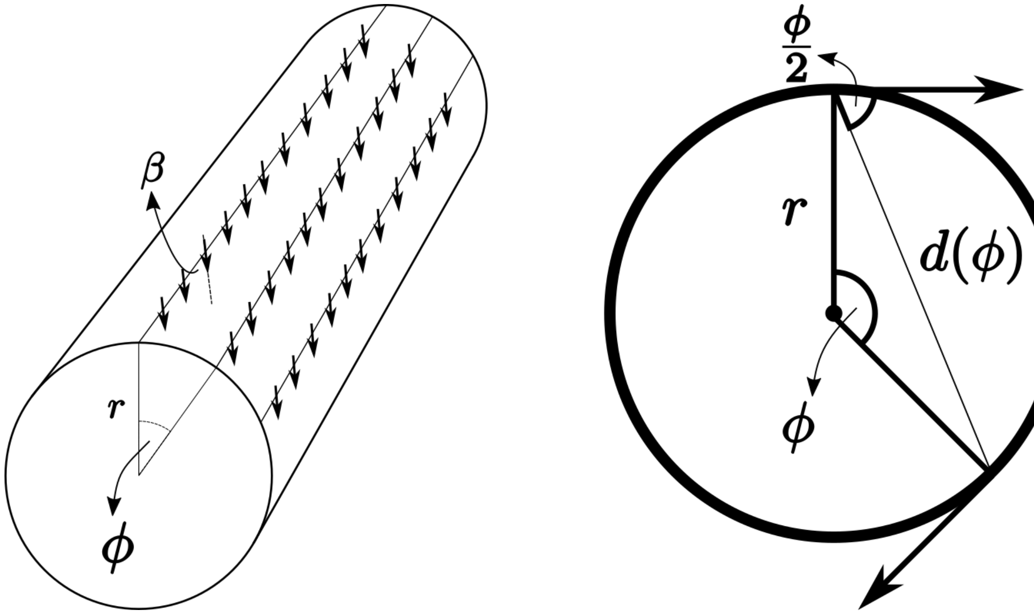


FIG. S6. (Left) Schematics of a tubular aggregate. All the transition dipoles are making an angle $\beta$ with the tube axis. (Right) Cross section of the tube showing the configuration of two interacting stripes of dipoles.

Substituting the above back to Eq. (S31) we arrive at Eq. (6)

$$E(0,\pm1) - E(0,0) = \frac{2\pi\mu_0^2}{rA_0}\sin^2\beta \tag{S35}$$

## S9. FINITE TUBE EXTENSION OF EQ. (6) IN THE MAIN TEXT

In realistic situations one needs to take into account the finite lengths of the tubular systems. Under such considerations Eqs. (S33) and (S34) should be revised as [1]

$$J_{\parallel}(x,L,\phi) = \frac{2}{L}\left(\frac{1}{L} - \frac{1}{\sqrt{x^2+L^2}}\right)\cos^2\beta - \frac{2L}{x^2\sqrt{x^2+L^2}}\sin^2\beta\cos^2\frac{\phi}{2} \tag{S36}$$

$$J_{\perp}(x,L,\phi) = \frac{2(\sqrt{x^2+L^2}-x)}{x^2L}\sin^2\beta\sin^2\frac{\phi}{2} \tag{S37}$$

Substituting the above expressions into Eq. (S31), the results are numerically evaluated and divided by the corresponding infinite tube values, as presented in Fig.S7 for different $\beta$ values as functions of the tube radius-to-length ratio $r/L$.

While in the long tube limit ($r/L \to 0$) we recover the infinite tube result, Eq. (S35), for small $\beta$ the deviation can be significant. This derives from the term proportional to $\cos^2\beta$

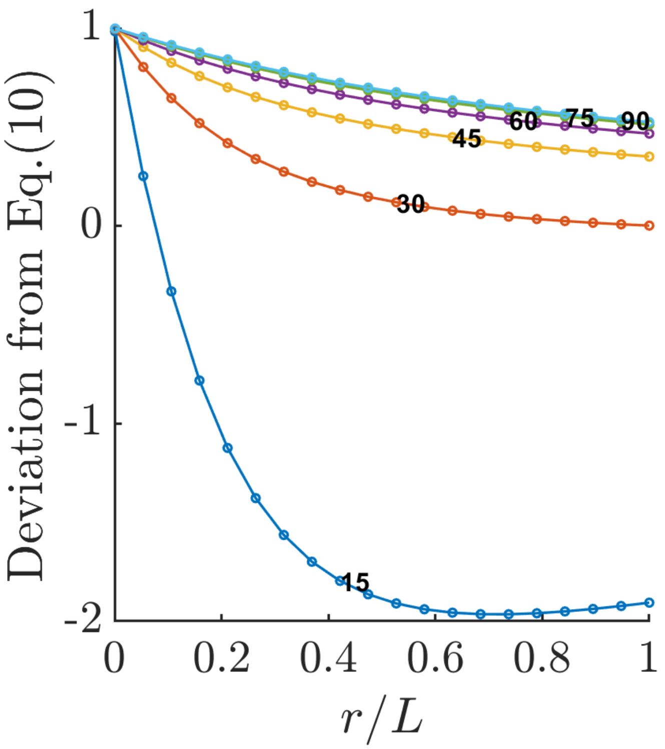


FIG. S7. Numerical integration of Eq. (S31) for finite tubes. From the bottom curve to the top: $\beta$ = 15, 30, 45, 60, 75, and 90 degrees. The results are presented as the relative values to the infinite tube expression Eq. (S35).

in Eq. (S36) which becomes significant for small $L$. In fact the relative position of the two perpendicular and the parallel peaks is reversed compared to the infinite tube for such cases.

## S10. UNIVERSALITY OF POWER-LAW EXPONENTS OF DOS AND $T$-DEPENDENT LINEWIDTH IN MOLECULAR THIN FILMS

In Fig. S8 we show the fitted power-law exponents of the DOS and the $T$-dependent homogeneous absorption linewidth as functions of lattice parameters of close-packed C8S3 dyes on a plane. The numerical results agree well with both the dipole square lattice models and the continuum model discussed in the main text [$E^{0.5}$ for the DOS and $W(T) \propto T^{s+1.5}$, where $s = 3$ represents the scaling of the cubic super-Ohmic bath spectral density]. This result is also consistent with the simulation of tubular C8S3 dye aggregates presented in Fig. 4 of the main text. The relation between dipole tubes and planes is discussed in the

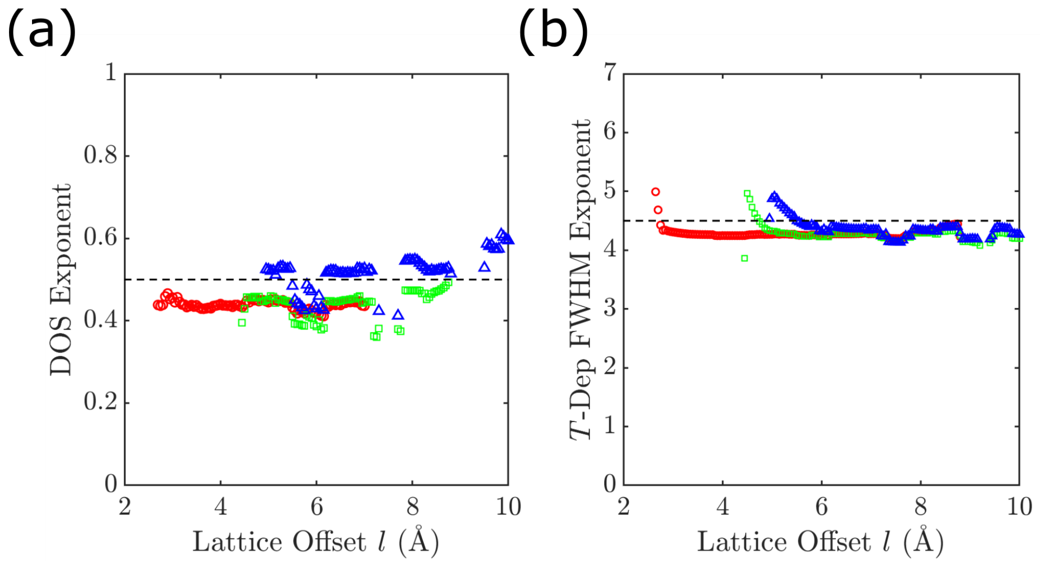


FIG. S8. (a) The fitted power-law exponents of the exciton DOS as functions of the brick wall lattice offset of planar aggregates. See the inset of Fig. 4(a) for illustration of the lattice. (b) The fitted power-law exponents of the $T$-dependent linewidth of the same systems as in (a).

next section in more details.

## S11. RADIUS DEPENDENCE OF $T$-DEPENDENT LINEWIDTH OF TUBULAR DIPOLAR SYSTEMS: 1D TO 2D TRANSITION

It has been shown that the transport properties of a tubular system along its axis scale between the 1D and the 2D limits as functions of radius.[11] The order parameter in this context is the ratio between the localization length $\xi$ and the radius $r$: For $\xi/r \gg 1$, the quasi-particle (Frenkel excitons in the present paper) wavefunction remains its phase coherence across the circumference of the tube. On the other hand, for $\xi/r \ll 1$, the quasi-particle wavefunction is strongly localized and its transport character is equivalent to that of a 2D lattice.

In terms of the scaling of DOS at the band edge, one expects a transition from the $E^{-0.5}$ scaling of 1D systems to the $E^{0.5}$ scaling discussed in the main text with increasing tube radius. This is confirmed in Fig. S9 where we examine the $T$-dependent linewidth power-law exponent as a function of tube radius. Here we take a square lattice wrapped onto cylindrical shape as shown in Fig. S6(a) with $R$ sites in the circumference and $\beta = \pi/4$. For this series

of systems, one recovers the $E^{-0.5}$ scaling DOS of 1D systems when $R$ is small and the $E^{0.5}$ scaling for 2D systems with large $R$. Following Eq. (4) in the main text, one expects the power-law exponent of $T$-dependent absorption linewidth to scale between 3.5 (1D) and 4.5 (2D) for a cubic super-Ohmic bath, as can be seen in Fig. S9. This is in agreement with the absorption lineshape simulations of tubular dye aggregates by Knoester et al.[12] and suggests that the tubes studied therein are in or approach the 2D limit.

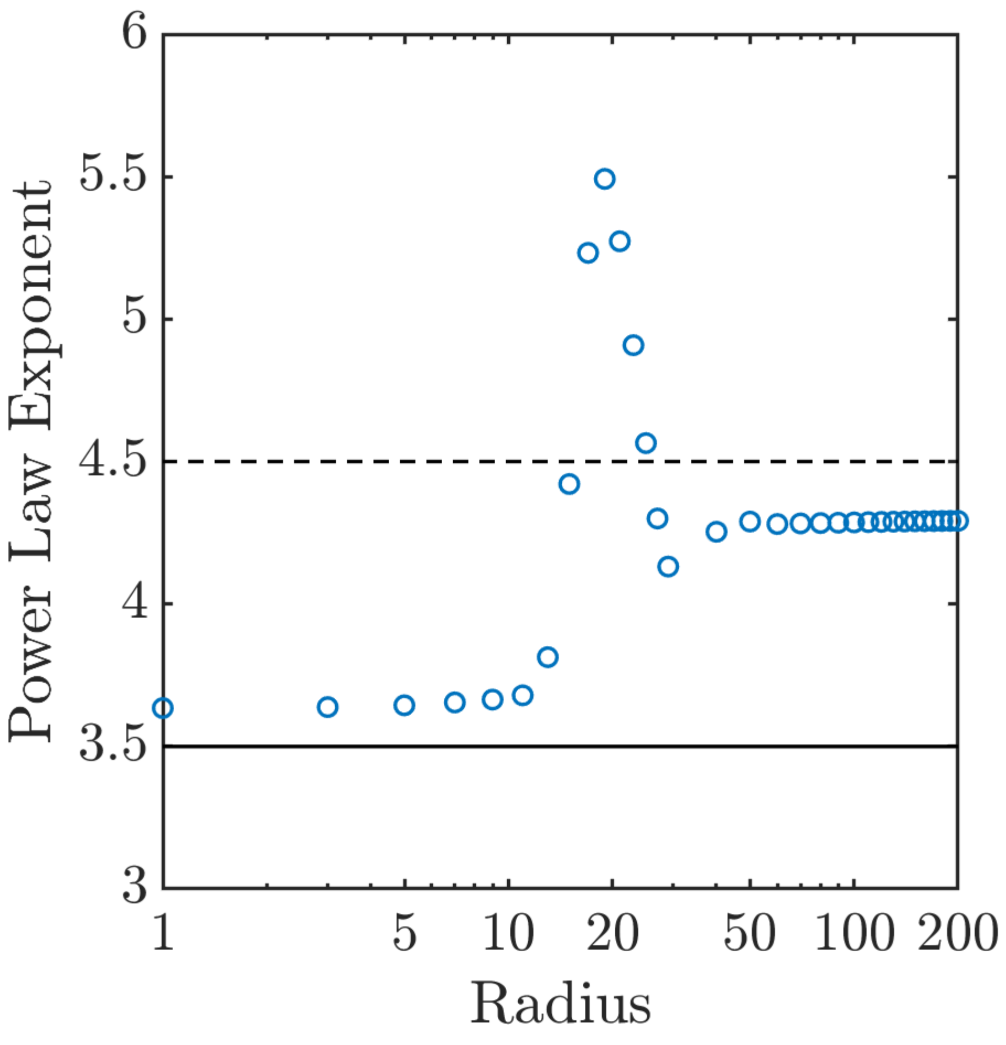


FIG. S9. The power-law exponents of the $T$-dependent homogeneous linewidth as a function of tube radius. A cubic super-Ohmic bath spectral density is used $\lim_{\omega \to 0} J(\omega) \propto \omega^3$. The solid line indicates the 1D limit, a $T^{3.5}$ scaling, and the dashed line indicates the 2D limit, a $T^{4.5}$ scaling. The peak around $R = 20$ is attributed to the deviation from power-law form in the transition regime.

[1] C. Chuang, J. Knoester, and J. Cao, J. Phys. Chem. B **118**, 7827 (2014).

[2] P. L. C. Y. B. Gaididei, M. Johansson, K. O. Rasmussen, V. K. Mezentsev, and J. J. Rasmussen, Phys. Rev. B **57**, 11303 (1998).

[3] M. L. Glasser, Journal of Mathematical Physics **14**, 409 (1973).

[4] L. D. Bakalis, I. Rubtsov, and J. Knoester, J. Chem. Phys. **117**, 5393 (2002).

[5] V. Czikkely, H. D. Försterling, and H. Kuhn, Chem. Phys. Lett. **6**, 11 (1970).

[6] K. A. Kistler, F. C. Spano, and S. Matsika, J. Phys. Chem. B **117**, 2032 (2013).

[7] M. J. Frisch, G. W. Trucks, H. B. Schlegel, G. E. Scuseria, M. A. Robb, J. R. Cheeseman, G. Scalmani, V. Barone, G. A. Petersson, H. Nakatsuji, X. Li, M. Caricato, A. V. Marenich, J. Bloino, B. G. Janesko, R. Gomperts, B. Mennucci, H. P. Hratchian, J. V. Ortiz, A. F. Izmaylov, J. L. Sonnenberg, D. Williams-Young, F. Ding, F. Lipparini, F. Egidi, J. Goings, B. Peng, A. Petrone, T. Henderson, D. Ranasinghe, V. G. Zakrzewski, J. Gao, N. Rega, G. Zheng, W. Liang, M. Hada, M. Ehara, K. Toyota, R. Fukuda, J. Hasegawa, M. Ishida, T. Nakajima, Y. Honda, O. Kitao, H. Nakai, T. Vreven, K. Throssell, J. A. Montgomery, Jr., J. E. Peralta, F. Ogliaro, M. J. Bearpark, J. J. Heyd, E. N. Brothers, K. N. Kudin, V. N. Staroverov, T. A. Keith, R. Kobayashi, J. Normand, K. Raghavachari, A. P. Rendell, J. C. Burant, S. S. Iyengar, J. Tomasi, M. Cossi, J. M. Millam, M. Klene, C. Adamo, R. Cammi, J. W. Ochterski, R. L. Martin, K. Morokuma, O. Farkas, J. B. Foresman, and D. J. Fox, "Gaussian˜16 Revision C.01," (2016), gaussian Inc. Wallingford CT.

[8] C. Didraga, J. A. Klugkist, and J. Knoester, J. Phys. Chem. B **106**, 11474 (2002).

[9] G. Dresselhaus, S. Riichiro, *et al.*, *Physical properties of carbon nanotubes* (World scientific, 1998).

[10] J. Sperling, A. Nemeth, J. Hauer, D. Abramavicius, S. Mukamel, H. F. Kauffmann, and F. Milota, J. Phys. Chem. A **114**, 8179 (2010).

[11] C. Chuang, C. K. Lee, J. M. Moix, J. Knoester, and J. Cao, Phys. Rev. Lett. **116**, 196803 (2016).

[12] E. A. Bloemsma, S. M. Vlaming, V. A. Malyshev, and J. Knoester, Phys. Rev. Lett. **114**, 156804 (2015).
